# Supplementary material for: On the Regularity of Attention
Source: arXiv:2102.05628 source file (2021-02-10)
Supplement: Supplementary file 1 [file appendix_analysis.tex]

\section{Proofs From Section~\ref{sec:analysis}}\label{app:analysis_proofs}

% \james{$E$ is compact and $f\in Lip(1)\implies \|f\|_\infty < \infty$, (WLOG, it can be taken $<diam(E)$) so the same proof applies for 1-wasserstein distnace, eliminating the need for a corollary.}
\begin{lemma}\label{lem:psi_cont}
	Let $\nu\in \calP(E)$ be fixed, where $E\subset\R^d$ is compact. The mapping $\Psi_\bdot(\nu):L^1(\nu)\to (\calP_1(E),\W_1)$ is continuous.
\end{lemma}
\begin{proof}
	Suppose $\{F_n\}\subset L^1(\nu)$ converges to $G\in L^1(\nu)$, and let $f\in Lip(1)$. Then
	\begin{align*}
			|\Psi_G(\nu)(f) - \Psi_{F_n}(\nu)(f)| &= \left|\frac{\int f(x) G(x)\nu(\dd x)}{\nu(G)} - \frac{\int f(x)F_n(x) \nu(\dd x)}{\nu(F_n)}\right|\\
			&= \left|\int \left[\frac{G(x)}{\nu(G)} - \frac{F_n(x)}{\nu(F_n)}\right]f(x)\nu(\dd x)\right|\\
			&\leq \left\|\frac{G}{\nu(G)} - \frac{F_n}{\nu(F_n)}\right\|_{L^1(\nu)}\|f\|_\infty\\
			&\leq \left\|\frac{G}{\nu(G)} - \frac{F_n}{\nu(F_n)}\right\|_{L^1(\nu)} \diam(E).
		\end{align*}
		In the last line, we used the fact that $\Psi_{G}(\nu)(\bar{f}) = \Psi_{F_n}(\nu)(\bar{f})$ for any constant function $\bar{f}$. This allows us to subtract from $f$ any constant without changing the value of $|\Psi_{G}(\nu)(f) - \Psi_{F_n}(\nu)(f)|$. Hence, we can assume without loss of generality that $\|f\|_{\infty} \leq \diam(E)$ (picking an arbitrary $x \in E$, we have $\forall y \in E$, $|f(y) - f(x)| \leq |y - x| \|f\|_{Lip} \leq \diam(E)$).
		Taking the supremum over $f$ gives us $\W_1(\Psi_G(\nu), \Psi_{F_n}(\nu)) \leq \left\|\frac{G}{\nu(G)} - \frac{F_n}{\nu(F_n)}\right\|_{L^1(\nu)}$. Letting $n \to \infty$ concludes the proof.
\end{proof}
% \begin{corollary}\label{coro:psi_cont}\james{checked}
% 	Since $\W_1(\mu,\nu)\leq \diam(E)\|\mu-\nu\|_{TV}$ (see \cite{villani2008optimal}), $\Psi_\bdot(\nu)$ is also continuous in the 1-Wasserstein topology.
% \end{corollary}

\begin{lemma}[\cite{himmelberg1976optimal}, Theorem 2]\label{lem:himmel1}
	Let $S$ and $A$ be Borel spaces, and $R$ be a Borel measurable compact-valued multi-function from $S\to A$ (i.e. $\forall s\in S, R(s) \subset A$ and is compact). With $GrR = \{(s,a) \in S\times A | a \in R(s)\}$, we let $u:Gr R\to \R$ be a Borel measurable function such that $u(s,\bdot)$ is an u.s.c. function on $R(s)$ for each $s\in S$. Then, there exists a Borel measurable selector $f:S\to A$ for $R$ such that
	\[
		u(s, f(s)) = \max_{a\in R(s)}u(s,a)~\forall s\in S.
	\]Moreover, the function defined by $v(s)=\max_{a\in R(s)}u(s,a)$ is Borel measurable.
\end{lemma}

% \begin{lemma}[\cite{himmelberg1976optimal}, Theorem 3]\label{lem:himmel2}
% 	Let $S$ and $A$ be Borel sapces and $F$ a multifunction from $S\to A$ with compact values. Then the following are equivalent:
% 	\begin{enumerate}
% 		\item $F$ is Borel measurable;
% 		\item $F^{-1}(U)$ is a Borel set for every open $U\subset A$;
% 		\item $Gr F=\{(s,a)\st a\in F(s)\}$ is a Borel subset of $S\times A$;
% 		\item $F$ is a Borel measurable function from $S$ to the space $cpt(A)$ of compact subsets of $A$ topologized by the Hausdorff metric.
% 	\end{enumerate}
% \end{lemma}

\begin{lemma}[\cite{van2014renyi}, Theorem 19]\label{lem:kl_usc}
	Suppose that $\calX$ is a Polish space (which is true for $E$ in particular). Then for $P,Q\in \calP(\calX)$, $\KL(P\|Q)$ is a lower semi-continuous function of the pair $(P,Q)$ in the weak topology.
\end{lemma}

\begin{lemma}[\cite{aliprantis2013infinite}, Th. 18.17 p.603 (Filippov's Implicit Function Th)]\label{lem:filippov}
	Let $(S,\Sigma)$ be a measurable space and let $X,Y$ be separable measurable spaces. Suppose that $f:S\times X\to Y$ is a Carath\'eodory function and that $\vphi:S\to X$ is a weakly measurable correspondence with nonempty compact values. Assume that $\pi:S\to Y$ is a measurable selector from the range of $f$ on $\vphi$ in the sense that $\pi$ is measurable and for each $s\in S$ there exists $x\in \vphi(s)$ with $\pi(s)=f(s,x)$. Then the correspondence $\nu:S\to X$ defined by
	\[
		\nu(s) = \{x\in\vphi(s)\st f(s,x) = \pi(s)\}
	\]is measurable and admits a measurable selector, i.e. in addition to being measurable, there is a measurable function $\xi:S\to X$ s.t. $\xi(s)\in \nu(s)$ i.e. $\pi(s)=f(s,\xi(s))$ for each $s\in S$.
\end{lemma}

\label{proof:maxent}
\maxent*
\begin{proof}
	
	For the existence and uniqueness of the maximum entropy distribution, let $\gamma\in \calQ(\nu,x)$ be any other measure, and denote by $m(x):=\diff{\mu^*_x}{\nu}$ and $n(x):=\diff{\gamma}{\nu}(x)$. Then
	\begin{align*}
	 	H_\nu(\gamma)&= -\int n(y)\log n(y)\nu(\dd y) \\
	 	&= -\int n(y)\log \frac{n(y)}{m(y)}\nu(\dd y) - \int n(y)\log m(y)\nu(\dd y)\\
	 	&=- \KL(\gamma\|\mu^*_x) - \int n(y)\log m(y)\nu(\dd y)\\
	 	&=- \KL(\gamma\|\mu^*_x) - \int n(y)[\ip{\lambda(x)}{k(x,y)} - A(x)]\nu(\dd y)\\
	 	&=- \KL(\gamma\|\mu^*_x) - \int [\ip{\lambda(x)}{k(x,y)} - A(x)]\gamma(\dd y)  \\
	 	&=- \KL(\gamma\|\mu^*_x) - [\ip{\lambda(x)}{f(x)} - A(x)] & \text{by linearity and }\gamma \in \calQ(\nu,x) \\
	 	&=- \KL(\gamma\|\mu^*_x) - \int [\ip{\lambda(x)}{k(x,y)} - A(x)]\mu^*_x(\dd y) & \text{by linearity and }\mu^*_x \in \calQ(\nu,x)\\
	 	&=- \KL(\gamma\|\mu^*_x) + H_{\nu}(\mu^*_x)\\
	 	&\leq H_\nu(\mu^*_x).
 	\end{align*} 		
 	since $\KL(\nu\|\mu^*_x)\geq 0$ and where $A(x) = \log \int \exp \ip{\lambda(x)}{k(x,y)}\nu(\dd y)$. This proves that $\mu^*_x$ is indeed the maximum entropy distribution, and is unique since any other maximum verifies $\KL(\gamma\|\mu^*_x) = 0$.

	The second statement is effectively a measurable selection theorem, for which we will apply Lemma~\ref{lem:himmel1} with:
	\begin{itemize}
	    \item $S = E$ and $A = \calP(E)$,
	    \item $R(x) = \calQ(\nu,x) \subset \calP(E)$ ($\nu$ is fixed throughout this theorem and its proof), and
	    \item $u(x,\mu) = H_\nu(\mu) = - \KL(\mu\|\nu) \in \R$ for $\mu \in \calQ(\nu,x)$.
	\end{itemize}
	
	First, $S = E$ is straightforwardly a Borel space. As far as $A$ is concerned, we are working on the 1-Wasserstein space $\calW_1=(\calP_1(E),\W_1)$, which is a complete metric space since $E\subset\R^d$ and $E$ is equipped with the Borel $\sigma$-algebra, hence $A = \calP(E)$ is also Borel.

	Second, by Lemma~\ref{lem:kl_usc}, $\mu \mapsto H_\nu(\mu) = -\KL(\mu\|\nu)$ is u.s.c. on $\calQ(\nu,x)$ for each $x\in E$. This implies in particular that $H_\nu^{-1}(]-\infty,a[)$ is open in the weak (i.e. 1-Wasserstein) topology for any $a$. Since the rays $]-\infty,a[$ generate the Borel sets, we get that $u$ is Borel-measurable.
    
	 In order to apply Lemma~\ref{lem:himmel1}, we need to prove that $R = x\mapsto \calQ(\nu,x)$ is measurable and compact-valued. This will conclude the proof as Lemma~\ref{lem:himmel1} guarantees that the selector, which corresponds to $x \to \mu_x^*$, is measurable.

	Let us thus prove that $x\mapsto \calQ(\nu,x)$ is measurable and compact-valued. Define $AC(\nu):=\{\mu\in \calW_1\st \mu \ll \nu\}$ and the mapping $\phi:E\times \calW_1\to E$ by $\phi(x,\mu)=\mu(k(x,\bdot))$; we can describe $\calQ(\nu,x)$ as the following:
	\[
		\calQ(\nu,x)=AC(\nu)\cap \{\mu\in \calW_1\st \phi(x,\mu)=f(x)\}.
	\]We will show that $AC(\nu)$ is measurable and closed in $\calW_1$, and that ${x \mapsto\{\mu\in \calW_1\st \phi(x,\mu)=f(x)\}}$ is a measurable, closed-valued correspondence, yielding the result. 

	For the first step, we have that $\{\mu = \Psi_X(\nu) \st X\in L^1(\R_{+};\nu)\}\subset AC(\nu)$. Conversely, $\mu\in AC(\nu)\implies \exists X\in L^1(\R_{+};\nu)$ s.t. $\mu(\dd x) = \Psi_X(\nu)$ by the Radon-Nikodym Theorem. Therefore, $AC(\nu) = \{\Psi_X(\nu)\st X\in L^1(\R_{+};\nu)\}$. Moreover, by Lemma~\ref{lem:psi_cont}, $X\mapsto \Psi_X(\nu)$ is a continuous map from $L^1(\R_+;\nu)\to \calW_1$, therefore $AC(\nu)$, which is the image of $L^1(\R_{+};\nu)$ under $\Psi_\bdot(\nu)$, is Borel measurable. Moreover, as $L^1(\R_{+};\nu)$ is closed, $AC(\nu)$ is also closed.

	For the second step, we apply Lemma~\ref{lem:filippov}. $\phi:E\times \calW_1\to E$ is a Caratheodory function. Indeed, $\forall \mu$, $x\mapsto\phi(x,\mu)$ is measurable by Fubini's Theorem, and $\forall x$, $\mu\mapsto \phi(x,\mu)$ is continuous in the weak (i.e. Wasserstein) topology. The correspondence from Lemma~\ref{lem:filippov}, $\vphi:E\to \calW_1$, is the constant correspondence $\vphi(x)=\calW_1$. The selector $\pi:E\to E$ is the function $f:E\to E$ which is measurable by assumption. Therefore, by Lemma~\ref{lem:filippov}, the level-set correspondence
	\[
		x\mapsto \{\mu \st \phi(x,\mu)=f(x)\}
	\]is measurable. Moreover, $\{f(x)\}$ is a closed set, and $\mu\mapsto \phi(x,\mu)$ is continuous so  $\phi(x,\bdot)^{-1}(\{f(x)\})$ is a closed set. This proves that $\calQ(\nu,x)$ is closed in $\calW_1$. Since $\calW_1$ is compact by compactness of $E$ \cite[ Ch 6]{villani2008optimal}, we have shown that $\calQ(\nu,x)$ is compact which concludes the proof.
\end{proof}

\label{proof:expmomproj}
\expmomproj*
\begin{proof} This proof is straightforward and follows the lines of \cite{koller2009probabilistic}, Theorem 8.6.
	Let $\theta_M=\mu(F)$ so that $\nu_{\theta_M}\in \calF$ is the measure which satisfies
	\[
		\nu_{\theta_M}(F) = \mu(F)
	\]and let $\nu_\theta$ be any other element of $\calF$. Then,
	\begin{align*}
		\KL(\mu\|\nu_{\theta_M}) - \KL(\mu\|\nu_\theta) &= \int \log \diff{\mu}{\nu_{\theta_M}}\dd \mu - \int \log \diff{\mu}{\nu_\theta}\dd \mu\\
		&= \int \log\diff{\nu_\theta}{\nu_{\theta_M}}\dd \mu\\
		&= \int \log \exp(\ip{\theta_M - \theta}{F(x)})\dd \mu(x) - \log\frac{\calZ(\theta_M)}{\calZ(\theta)}\\\
		&= \int \ip{\theta_M - \theta}{F(x)}\dd \mu(x) - \log\frac{\calZ(\theta_M)}{\calZ(\theta)}\\
		&= \ip{\theta_M-\theta}{\mu(F)} -  \log\frac{\calZ(\theta_M)}{\calZ(\theta)}\\
		&= \ip{\theta_M - \theta}{\nu_{\theta_M}(F)} - \log\frac{\calZ(\theta_M)}{\calZ(\theta)}\\
		&= - \KL(\nu_{\theta_M}\|\nu_\theta) \leq 0
	\end{align*}
	where $\calZ(\theta)=\exp(A(\theta))$ is the partition function.
\end{proof}

\begin{definition}[Measure Convolution]
	Let $\mu,\nu\in \calP(\R^d)$ be measures. Then we define the \defn{measure convolution} of $\mu$ and $\nu$, denoted $\mu*\nu$, by
	\[
		(\mu*\nu)(f) := \int f(x+y)\mu(\dd x)\nu(\dd y)~~~\forall f\in \calB_b(\R^d).
	\]
	\end{definition}

\begin{lemma}\label{prop:conv_stat}
	Let $\mu,\nu \in \calP(\R^d)$, and assume that $F:\R^d \to \R$ is a measurable, linear function, with the additional stipulation that $F\in L^1(\mu)\cap L^1(\nu)$. Then we have
	\[
		(\mu*\nu)(F) = \mu(F) + \nu(F).
	\]
\end{lemma}

\begin{proof}
We have:
    \begin{align*}
        (\mu*\nu)(F) &= \int F(x+y)\mu(\dd x)\nu(\dd y) = \int [F(x) + F(y)]\mu(\dd x)\nu(\dd y) \\ 
        &= \int F(x) \mu(\dd x)\nu(\dd y) + \int F(y)\mu(\dd x)\nu(\dd y) = \mu(F) + \nu(F),
    \end{align*}
which concludes the proof.

\end{proof}

\begin{lemma}\label{lem:conv_limit}
	Define $\rho_n:=\calN(0,\sigma^2_nI)$ be a multivariate Gaussian on $\R^d$, $\sigma_n\to 0$, and let $\mu\in\calP_1(\R^d)$. Then $\rho_n*\mu\in \calP_1(\R^d)$ and  $\W_1(\rho_n*\mu, \mu)\to 0$ as $n\to \infty$.
\end{lemma}
\begin{proof} Let $x_0 \in \mathbb{R}^d$.  A measure $\nu$ has finite 1st moment iif  $\int \|x_0 - x\| \nu(\dd x) < \infty$. 
Firstly, 
    \begin{align*}
        \int \|x_0 - x\| \rho_n*\mu(\dd x)&= \iint \|x_0 - (x + y)\|\rho_n(\dd x) \mu(\dd y) \\
        &\leq \iint (\|x_0/2 - x\| + \|x_0/2 - y\|)\rho_n(\dd x) \mu(\dd y)\\
        &\leq \int \|x_0/2 - x\|\rho_n(\dd x) + \int \|x_0/2 - y\|\mu(\dd y)<\infty
    \end{align*}
    so that $\rho_n*\mu\in \calP_1(\R^d)$. Now let $f\in Lip(1)$, then
	\begin{align*}
		|(\rho_n*\mu)(f) - \mu(f)| &= \left|\iint[f(x+y) - f(y)]\rho_n(\dd x)\mu(\dd y)\right|\\
		&\leq \iint |f(x+y) - f(y)|\rho_n(\dd x)\mu(\dd y)\\
		&\leq \int \|x+y-y\|\mu(\dd y)\rho_n(\dd x)\\
		&= \int \|x\| \rho_n(\dd x) \to \int \|x\| \delta_0(\dd x) = 0
	\end{align*}
	as $n\to \infty$. Since the upper bound is independent of $f$, we are done.
\end{proof}

\label{proof:deltamomproj}
\deltamomproj*
\begin{proof}
	Let $f:=\mu(F)$. Below, we extend $\mu\in \calP_1(E)$ to be a (compactly supported) element of $\calP_1(\R^d)$ by simply setting ${\mu(A)=\mu(A\cap E)~\forall A\in \calB(\R^d)}$, and trivially extend $F$ to $\R^d$.
	\begin{enumerate}
		\item We have that $\rho_n*\mu(F)=\mu(F)~\forall n$ by Lemma~\ref{prop:conv_stat} since $F(x)=x$ is linear and $\rho_n(F) = 0$. Therefore, $\Pi_\calF(\rho_n*\mu)=\Pi_\calF(\mu), \forall n$.
		\item Let $\calF_n$ be as above. %\remi{TODO Detail the exponential family + justify well-posedness of the projection on $\calF_n$. Define $f$ and $\nu$.} 
		By the previous step, we have 
		\[
			\Pi_{\calF_n}(\rho_n*\mu)  = \Pi_{\calF_n}(\mu) = (\rho_n*\nu)_f = \rho_n*\nu_f.
		\]Moreover, since $\rho_n*\mu\sim \nu~\forall \nu\in \calF_n$ and $\calF_n$ is an exponential family, by Proposition~\ref{prop:expmomproj}
		\[
			\Pi_{\calF_n}(\rho_n*\mu) = \arg\min_{\nu \in \calF_n}\KL(\rho_n*\mu\|\nu).
		\]
		\item Finally, $\nu_f := \Pi_{\calF}(\mu)$ is equal to the limit
		\[
			\nu_f \overset{(1)}{=}  \lim_{n\to \infty} \rho_n*\nu_f  \overset{(2)}{=} \lim_{n\to \infty}\Pi_{\calF_n}(\rho_n*\mu) \overset{(3)}{=}  \lim_{n\to \infty}\arg\min_{\nu\in \calF_n}\KL(\rho_n*\mu\|\nu)
		\]where (1) is due to Lemma~\ref{lem:conv_limit}, and (2), (3) are due to step 2. Hence we can think of $\nu_f$ as the limit of the minimizers in the 1-Wasserstein sense.
	\end{enumerate}
\end{proof}
